# Supplementary material for: Verifying C11-Style Weak Memory Libraries
Source: arXiv:2012.14133 source file (2020-12-28)
Supplement: Supplementary file 1 [file appendix.tex]

\newpage

\section{Appendix}

\begin{theorem} If $R$ is a forward simulation between $AO$ and $CO$,
  then for any client that only synchronises through $AO$ (and $CO$)
  we have $C[AO] \refby C[CO]$.
\end{theorem}
\begin{proof}[Proof (sketch)] %  Let $\Omega$ and $\Pi$ be configurations of
  % $C[AO]$ and $C[CO]$, respectively.
  % Let
  % $\widehat{R}(\Omega, \Pi) \equiv loc(\Omega)_{|C} = loc(\Pi)_{|A} \wedge
  % R(\st(\Omega), \st(\Pi))$ be a relation over full
  % configurations. 
  Given a trace of $C[CO]$, it is possible to construct a
  corresponding trace of $C[AO]$ using $R$. Correspondence between the
  initial states of $C[CO]$ and $C[AO]$ is trivial by the
  initialisation condition in \refsec{def:fsim}. For any purely local
  step of the client of $C[CO]$, the same step is available in
  $C[AO]$. For any read of a global variable in $C[CO]$, the same read
  is available in $C[AO]$ by the client observation property in
  \refdef{def:fsim}, and these update the local state in the same
  way. Moreover, since the client does not synchronise outside $CO$,
  the library states of $\Omega$ and $\Pi$ are equivalent. A similar
  argument applies to client writes. For each library transition, by
  the stuttering and non-stuttering step rules in \refdef{def:fsim},
  we have that $R$ holds in the post state (where the abstract may not
  have taken a step). Importantly, by the client observation we have
  the conditions required for \refdef{def:cont-refin-1}. Then, after
  removing stuttering, one obtains the required trace refinement
  relationship (\refdef{def:prog-ref}). Finally, since we chose the
  trace of $C[CO]$ arbitrarily, we obtain program refinement as
  defined in \refdef{def:prog-ref}. 
\end{proof}

\subsection{Sequence Lock}
\label{sec:sequence-lock}

The first example of our contextual refinement is the refinement of a
sequence lock. An implementation of the concrete sequence lock is
given in \reffig{seqlock_imp}. The lock operates over one shared
variable ($glb$). If {\bf Acquire} is invoked, it waits until
it sees an even value for $glb$ and then tries to increase the value
of $glb$ by one using a compare and swap (\textbf{CAS}) operation. If
the \textbf{CAS} is successful, then the lock is acquired, the outer
loop is terminated and the thread can enter its critical section. Once
the thread exits its critical section it should release the lock by
invoking {\bf Release} which will increase the value of $glb$ by
one making the last value written to the $glb$ an even number again.

We have implemented the $\kwcas(x,u,v)$ operation using the semantics
given in \reffig{fig:surrey-opsem} where a successful operation
(i.e. the operation observes a write with value $u$) is modelled by an
release-acquire update and the unsuccessful one (i.e. the operation
does not observe a write with value $u$) by a relaxed read.

It is worth noting that a successful $\kwcas$ operation is both
releasing and acquiring meaning that if it observes a releasing write
written by the release operation of the previous lock it synchronises
the acquiring thread with the thread previously holding the lock. The
operation could become more relaxed if the semantics provided an
acquiring-only update operation.

Following the forward simulation \refdef{def:fsim}, we provide a simulation relation between abstract lock object and the concrete the given implementation of sequence lock. For the client observation relation we have:
\begin{equation}
\begin{split}
  \forall t, x~. \tst (\gamma_C.\tview_t(x)) \ge  \tst (\gamma_A.\tview_t(x)) \land \gamma_C.\covered = \gamma_A.\covered \wedge 
  \gamma_C.\writes = \gamma_A.\writes
\end{split}
\label{seqlock-forwardsim_client}
\end{equation}
\noindent where $\gamma_A$ and $\gamma_C$ represent abstract and
concrete client states, respectively. We define $\lhd$ to be the
domain restriction operator where
$S \lhd R = \{(x, y) \in R \mid x \in S\}$, and use it to give the
following relation between abstract and concrete library states, where
$glb$ and $l$ are variables:
\begin{equation}
\begin{split}
&\forall w_c . ~~ w_c\in\beta.\OW(t,glb)~ \implies  (\exists w_a . \wrval(w_c) = \wrval(w_a)  \land w_a\in\alpha.\OW(t, l) \\
 &\land (\GVar_C \lhd \beta.\mview_{w_c}) = (\GVar_C \lhd \alpha.\mview_{w_a})  \\
& \land \isReleasing(w_c) = \isReleasing(w_a) \land (w_c \in \beta.\covered \iff  w_a \in \alpha.\covered))
\end{split}
\label{seqlock-forwardsim}
\end{equation}

\noindent where $\beta$ is the concrete library state (the sequence
lock state in this case), $\alpha$ is the abstract object state, 
$\isReleasing$ is a predicate used to determine whether a
``synchronised read'' access of the corresponding parameter induces a
synchronisation.

We observe that the ${\bf Acquire}$ operation can successfully acquire
the lock only if the $\kwcas$ on line~2 is successful. Therefore in
order to prove the refinement, we will need to prove that whenever the
$\kwcas$ operation is successful, the abstract object can also
successfully acquire the lock maintaining the simulation relation.
Also the read on line 1 and the unsuccessful $\kwcas$ are stuttering
steps and we need to show that when those steps are taken the abstract
state remains unchanged and the new concrete state preserves the
simulation relation. The ${\bf Release}$ operation contains only one
releasing write on variable $glb$ which is considered to be a refining
step. It is straightforward to show that this operation refines the
abstract object release operation.

\begin{lemma}
  Relations (\ref{seqlock-forwardsim_client}) and
  (\ref{seqlock-forwardsim}) together form a forward simulation for
  synchronisation-free clients (\refdef{def:fsim}) between the abstract
  lock object and the sequence
  lock. % and the sequence lock therefore the concrete
  % implementation is a refinement of the abstract object lock.
\end{lemma}
\begin{proof} In Isabelle~\cite{Mech}.
\end{proof}

%\begin{lemma} The $SeqLock.Acquire()$ operation refines the abstract object $acquire()$ operation.
%\end{lemma}
%\begin{proof}Proof in Isabelle.
%\end{proof}
%

  \begin{figure*}[t]
    \hfill
    \begin{minipage}[b]{0.45\textwidth}
      $\textbf{Init:} \ \ glb = 0$
      \\[2pt]
      \begin{minipage}[t]{\textwidth}
        \small \textbf{Acquire()}:
        \begin{algorithmic}[1] \small
          \Statex \textbf{do}
          \Statex \quad \textbf{do}
          \State \quad \quad $r \leftarrow^{A} glb$ 
          \Statex \quad \textbf{until} $(even (r))$
          \State \quad $loc \gets \kwcas(glb, r, r+1)$ 
          \Statex \textbf{until} $(loc)$
        \end{algorithmic}
      \end{minipage}
      \\[5pt]
      \begin{minipage}[t]{\textwidth}
        \small \textbf{Release()}: 
        \begin{algorithmic}[1] \small
          \State $glb :=^{R} r + 2$ 
        \end{algorithmic}
      \end{minipage}
      \vspace{-1em}
      \caption{Implementation of a Sequence Lock}
      \label{seqlock_imp}
    \end{minipage}
    \hfill
    \begin{minipage}[b]{0.45\textwidth}
      $\textbf{Init:} \ \ nt = 0, \ \ sn = 0$\\[2pt]
      \begin{minipage}[t]{\columnwidth}
        \small \textbf{Acquire()}:
        \begin{algorithmic}[1] \small
          \State $my\_ticket \leftarrow \kwfai(nt)$
          \Statex  \textbf{do}
          \State  \quad $serving\_now \leftarrow^{A} sn$ 
          \Statex  \textbf{until} $(my\_ticket = serving\_now)$
        \end{algorithmic}
      \end{minipage}
      \\[5pt]
      \begin{minipage}[t]{\columnwidth}
        \small \textbf{Release()}: 
        \begin{algorithmic}[1] \small
          \State $sn :=^{R} serving\_now + 1$ 
        \end{algorithmic}
      \end{minipage}
      \vspace{-1em}
      \caption{Implementation of a Ticket Lock}
      \label{ticketlock_imp}
    \end{minipage}
    \hfill
\end{figure*}

\subsection{Ticket Lock}
\label{sec:ticket-lock}
Our second case study is the refinement of an implementation of a
ticket lock (given in Figure \ref{ticketlock_imp}). Unlike the
previous example, the ticket lock has two shared variables $nt$ (next
ticket) and $sn$ (serving now). Invocation of {\bf Acquire} loads the
next available ticket into a local register ($my\_ticket$) and
increases the value of $nt$ by one using a fetch-and-increase
($\kwfai$) operation. It then enters a busy loop and reads $sn$ until
it sees its own ticket value in $sn$ before it can enter its critical
section.

Similar to $\kwcas$, the $\kwfai(x)$ operation is defined using the basic operations of the semantics given in \reffig{fig:surrey-opsem}. The operation reads the value of  variable $x$, increases it by one and returns the old value. The operation is defined using a release-acquire update and forces a synchronisation if it reads from a releasing write on $x$. In the implementation of the ticket lock, the $\kwfai$ operation does not need to be synchronising and could be relaxed if the semantics supported a relaxed update. While defining a relaxed update is straightforward, it falls outside the scope of this work. Lock synchronisation should only happen when the lock is acquired by reading a value of $sn$ which is equal to $my\_ticket$ on line 2.

Here, like the previous example, we provide a simulation relation between abstract lock object and the concrete implementation. The client observation relation is the same as (\ref{seqlock-forwardsim_client}) given in the previous section. We give the following relation between abstract and concrete ticket lock states:
\begin{equation}
\begin{split}
\forall~wnt~wsn~. &~~(wnt\in \beta.\writeson(nt)\land 
cls.pc_t\in~\{1,2\}~\\
& \land 
wsn\in \beta.\OW(t,sn)
\land ~\wrval(wnt)~=~\wrval(wsn))~\implies~ \\
& (\exists~wl~.~wl\in\alpha.\OW(t,l)~\land ~even~(\wrval(wl))~\land wl \notin \alpha.\covered\\
&\land ~(\GVar_C \lhd \beta.\mview_{wsn}) = (\GVar_C \lhd \alpha.\mview_{wl}) 
\land  \isReleasing(wsn) = ~\isReleasing(wl))
\end{split}
\label{ticketlock-simrel}
\end{equation}
\noindent where $\writeson(x)$ is the set of writes on variable $x$,
$\beta$ is the concrete library state, and $\alpha$ is the abstract
object state.  % \bd{Give explanation of these conditions.}

If the read on line 2 of the {\bf Acquire} operation reads from a
write which its value is equal to the value of $my\_ticket$, then the
lock is acquired. Therefore we will need to show that if this
situation arises, the abstract lock object can also take an step and
successfully acquires the lock. We consider the $\kwfai$ operation on
line 1 and the read on line 2 if it reads a value that is not equal to
$my\_ticket$ to be a stuttering step. We prove that each of the
stuttering and non-stuttering steps preserves the simulation
relation. Similar to the previous example, the {\bf Release} operation
consists of only one releasing write to variable $sn$ and it is
straightforward to show that this operation refines the abstract
release operation.

\begin{lemma}
  Relations (\ref{seqlock-forwardsim_client}) and
  (\ref{ticketlock-simrel}) % are a forward simulation between the
  % abstract lock object and the ticket lock therefore the concrete
  % implementation is a refinement of the abstract object lock.
  together form a forward simulation for synchronisation-free clients
  (\refdef{def:fsim}) between the abstract lock object and the
  sequence lock.
\end{lemma}
\begin{proof} In Isabelle~\cite{Mech}.
\end{proof}

%%% Local Variables:
%%% mode: latex
%%% TeX-master: "main"
%%% End:
